# Supplementary material for: Towards Continuous Assurance Case Creation for ADS with the Evidential Tool Bus
Source: arXiv:2403.01918 source file (2024-03-04)
Supplement: Supplementary file 1 [file appendices.tex]

\appendices
\newpage
\onecolumn
\section{Top-level Assurance Pattern}
\label{app:datalogWorkflow}
